# Supplementary material for: CLINICSUM: Utilizing Language Models for Generating Clinical Summaries from Patient-Doctor Conversations
Source: arXiv:2412.04254 source file (2024-12-05)
Supplement: Supplementary file 1 [file appendix.tex]

\subsection{Fine-tuning Details}
\label{fine-tuning-details}
Table \ref{hyperparams_ft} outlines the hyper-parameters used to fine-tune the PLMs in our research, including LLMA-3-8B, Gemma-2-9B, Mistral-7B, and Mistral-Nemo instruct models. To ensure a fair comparison for the summary generation task, we applied the same hyper-parameters across all models. 

\begin{table}[ht]
\centering
\scriptsize
\caption{An overview of Hyper-parameters used to fine-tune PLM in \framework. }
\label{hyperparams_ft}
\begin{tabular}{l|l|p{3.5cm}}
\hline
\textbf{Hyperparameter}         & \textbf{Value} & \textbf{Summary}                                      \\ \hline
max\_seq\_length                & 2048           & truncate output sequences to this max length          \\ %\hline
prompt                          & alpaca prompt & instruction text prepended to all inputs              \\ %\hline
r                               & 16             & rank of the low-rank adaptation matrices              \\ %\hline
lora\_alpha                     & 16             & scaling factor applied                                \\ %\hline
lora\_dropout                   & 0              & 0 indicates all weights are considered                \\ %\hline
packing                         & FALSE          & each example is treated independently during training \\ %\hline
bias                            & none           & restricts additional bias in LORA layers              \\ %\hline
per\_device\_train\_batch\_size & 2              & batch size for training per device                    \\ %\hline
gradient\_accumulation\_steps   & 4              & \# of steps to accumulate gradients in training       \\ %\hline
use\_gradient\_checkpointing    & TRUE           & enables gradient checkpointing                        \\ %\hline
warmup\_steps                   & 5              & number of warmup steps during training                \\ %\hline
num\_train\_epochs              & 3              & model will train on the dataset three times           \\ %\hline
lr\_scheduler\_type             & linear         & linear scheduler decreases learning rate linearly     \\ %\hline
fp16                            & TRUE           & whether to use FP16 during training                   \\ %\hline
learning\_rate                  & 0.0002         & learning rate during training                         \\ %\hline
logging\_steps                  & 1              & specifies training log will be recorded once          \\ %\hline
optim                           & adamw\_8bit    & optimizer used during training                        \\ %\hline
weight\_decay                   & 0.01           & weights will be slightly penalized during training    \\ %\hline
seed                            & 3407           & sets the random seed for reproducibility              \\ \hline
\end{tabular}
\end{table}

Lora adapters of our fine-tuned models can be found in huggingface LLAMA-3-8B \footnote{https://huggingface.co/SubashNeupane/llama3-8b-SOAP\_summary-lora}, Mistral-Nemo-12B \footnote{https://huggingface.co/SubashNeupane/mistral-nemo-instruct-12-SOAP-summary-lora}, Mistral-7b-instruct
\footnote{https://huggingface.co/SubashNeupane/mistral-mistral-7b-instruct-SOAP-summary-lora}, Gemma-2-9b, 
\footnote{https://huggingface.co/SubashNeupane/gemma2-9b-SOAP\_Summary-lora} and LLAMA-3.1-8b
\footnote{https://huggingface.co/SubashNeupane/llama-3.1-8b-SOAP\_summary-lora}

\subsection{Token Count of Summaries}
\label{token_count_summaries}
Figure \ref{fig:tokens_summary} illustrates the total token count for 20 summaries produced by GPT-based models and fine-tuned models using our framework. Token counts for both GPT-based models  and open-source PLMs were computed using the \emph{BAAI/bge-large-en-v1.5} model from Hugging Face. Gemma-2-9B (average token count: 261.5) and LLAMA-3-8B (average token count: 260.15) align closely with the ground truth (average token count: 268.95) in terms of token counts, indicating their ability to generate concise and accurate summaries. In contrast, GPT-4-Turbo (average token count: 375.05) produced more tokens than the ground truth, highlighting a tendency toward verbosity or even hallucination. Mistral-Nemo (average token count: 291.55) and GPT-4-0-Mini (average token count: 281.25) also show increased token generation in some cases but have a tendency to generate fewer tokens, while Mistral-7B (average token count: 259.1) and GPT-3.5-Turbo (average token count: 237.65) generally produce fewer tokens, potentially missing critical details. Despite these variations, LLAMA-3-8B and Gemma-2-9B maintain a balanced approach of using and generating tokens that are strictly coherent with the context provided to them by retriever-based filtering, producing summaries that are aligned with the ground truth.
%This comparison highlights the critical role of token management in ensuring reliable summary performance.
\begin{figure*}
  \centering
  \includegraphics[width=1\linewidth]{figs/Grid 4.png}
  \caption{An illustration of total tokens count for 20 summaries generated by GPT-based and fine-tuned models.}
  \label{fig:tokens_summary}
\end{figure*}

\subsection{Instruction for SMEs}
\label{instruction_smes}
Please evaluate the summaries for the 20 provided patient-doctor conversations. The first column contains the conversations, while columns A and B present synthetically generated summaries. Column C contains the ground-truth summaries. If you prefer the summary in column A for a particular conversation, mark your preference as 'A'. If both summaries are equally good, mark your preference as 'A/B'. Your task is to select the best summary based on criteria such as factual accuracy, inclusion of critical and non-critical information, and exclusion of irrelevant details. A strong summary should be factually accurate, include all critical information, some non-critical information, and contain minimal irrelevant details. 

The definition of these  categories are as follows: 

\begin{itemize}
    \item \textbf{Factual Correctness} (our addition): Factual correctness ensures that the clinical summary accurately reflects the details of the patient-doctor conversation, including symptoms, diagnosis, and treatment. Errors or omissions in key facts can lead to misunderstandings and improper care. For example, for a given ground truth \emph{A 55-year-old female presents with shortness of breath and chest pain. She reports that the symptoms started two days ago. The doctor suspects a heart attack and orders an ECG. The patient has a history of hypertension and diabetes.} A good summary must capture all key factual information such as demographics, present illness, timeline of symptom, diagnosis, ordered test, and medical history.
    
    \item \textbf{Critical}: A good summary must include all critical information that are required for diagnosis and treatment plans. For example a consultation for a sudden vision could include key critical information including onset and duration of symptom, associated pain/ discomfort, recent trauma/injury, pre-existing condition like diabetes Presence of incorrect and incomplete information would be a medical risk.
    \item \textbf{Non-critical}: Non critical information are those that doesn't impact the medical value of of  summaries for example ``how many kids do you have'' for consultation of diabetes is not critical medically.
    \item \textbf{Irrelevant}: The absence of of irrelenat information does not impact the quality of summaries. For example the past medical history of sprained ankle can be deemed irrelevant during consultation of sudden loss of eyesight.
\end{itemize}

\subsection{Example of Inference using \framework}
Fig \ref{box:patient_doctor_conversation} presents an example of actual patient doctor conversation and Fig. \ref{box:summary_from_conversation} represents its clinical summary generated by \framework. 

\begin{tcolorbox}[colback=blue!5!white,colframe=blue!75!black,title=Patient-Doctor Conversation, breakable]
\footnotesize
\textbf{D:} Good morning! How can I help you today? \\
\textbf{P:} Hi, I've been experiencing shortness of breath for the past week and it's been bothering me. I thought I should come in and get it checked out. \\
\textbf{D:} I see. Shortness of breath can be concerning. Can you tell me more about your symptoms? How severe is the shortness of breath? \\
\textbf{P:} It's been moderate. I notice it especially when I exercise or engage in physical activities. \\
\textbf{D:} Okay. Have you noticed any other symptoms along with the shortness of breath? For example, do you hear any wheezing or have a cough? \\
\textbf{P:} Yes, I do hear wheezing when I breathe and sometimes I have a cough as well. \\
\textbf{D:} Thank you for sharing that information. Have you experienced similar symptoms in the past? \\
\textbf{P:} Yes, I had childhood asthma, but it hasn't bothered me much in recent years. \\
\textbf{D:} I see. It's important to consider your medical history. Does anyone in your family have a history of asthma or any other respiratory conditions? \\
\textbf{P:} Yes, my mother also had asthma. \\
\textbf{D:} That's helpful to know. Now, let's talk about any allergies you may have. Are you allergic to anything, such as pollen? \\
\textbf{P:} Yes, I am allergic to pollen. \\
\textbf{D:} Thank you for letting me know. Now, I'd like to perform a physical examination. I will listen to your lungs with a stethoscope to check for any abnormal sounds. Please take a deep breath in and out. \\
\textbf{P:} \textit{(takes a deep breath)} \\
\textbf{D:} I can hear wheezing on auscultation, which is consistent with your symptoms. To further evaluate your lung function, I would like to order a spirometry test. This will help us assess how well your lungs are functioning. \\
\textbf{P:} Okay, I'm willing to do the test. What does it involve? \\
\textbf{D:} During a spirometry test, you will be asked to take a deep breath and blow into a device called a spirometer. This device measures the amount of air you can exhale and how quickly you can do so. It's a simple and non-invasive test. \\
\textbf{P:} That sounds doable. When can I schedule the test? \\
\textbf{D:} We can schedule it for tomorrow morning. Before that, I would also like to rule out any other conditions that may present with similar symptoms. We will need to run some blood tests to check for any underlying causes. \\
\textbf{P:} Alright, I understand. I'll come in tomorrow for the spirometry test and blood tests. \\
\textbf{D:} Great. Once we have the results, we can discuss them together. Based on your symptoms, medical history, and physical examination findings, it is likely that you are experiencing an asthma exacerbation. However, we need to confirm this with the test results. \\
\textbf{P:} I appreciate your thoroughness. If it is asthma, what would be the treatment plan? \\
\textbf{D:} If the diagnosis confirms asthma, we will develop a personalized treatment plan for you. Since you mentioned that using an inhaler relieves your symptoms, we may prescribe a long-acting bronchodilator to help manage your symptoms on a daily basis. Additionally, we may recommend a short-acting bronchodilator to use as needed during episodes of shortness of breath. \\
\textbf{P:} That sounds reasonable. Will I need to make any lifestyle changes? \\
\textbf{D:} It's important to avoid triggers that may worsen your symptoms, such as exposure to allergens or irritants. Regular exercise is still beneficial, but we may need to adjust your routine to prevent asthma attacks. I also recommend getting an annual flu vaccine to reduce the risk of respiratory infections. \\
\textbf{P:} I will keep that in mind. Are there any potential side effects of the medications? \\
\textbf{D:} The most common side effects of bronchodilators are tremors, increased heart rate, and headache. However, these side effects are usually mild and temporary. We will monitor your response to the medication and adjust the dosage if needed. \\
\textbf{P:} That's good to know. Will I need to come in for regular check-ups? \\
\textbf{D:} Yes, regular follow-up appointments are important to monitor your asthma control and adjust the treatment plan if necessary. We will also provide education on proper inhaler technique and asthma management strategies. \\
\textbf{P:} I appreciate your guidance. I will make sure to schedule regular check-ups. Thank you for your help, doctor. \\
\textbf{D:} You're welcome. It's my pleasure to assist you. If you have any further questions or concerns, don't hesitate to reach out. Take care and I'll see you tomorrow for the tests. \\
\textbf{P:} Thank you, doctor. Goodbye. \\
\textbf{D:} Goodbye and take care. \\
\textbf{P:} Doctor, I have a few more questions before I leave. \\
\textbf{D:} Of course, please go ahead. \\
\textbf{P:} Will my asthma ever go away completely? \\
\textbf{D:} Asthma is a chronic condition, which means it usually lasts a lifetime. However, with proper management and treatment, you can control your symptoms and lead a normal life. \\
\textbf{P:} That's reassuring to know. Can I still exercise and participate in sports? \\
\textbf{D:} Absolutely! Regular exercise is important for overall health, and it can actually help improve lung function in people with asthma. We may need to adjust your medication or provide you with a pre-exercise bronchodilator to prevent exercise-induced symptoms. \\
\textbf{P:} That's good to hear. I enjoy being active, so I'm glad I can continue doing that. Are there any natural remedies or alternative treatments I can try? \\
\textbf{D:} While there are some alternative treatments that people with asthma may find helpful, it's important to remember that they should not replace prescribed medications. Some people find relief with techniques like breathing exercises, acupuncture, or herbal remedies, but it's best to discuss these options with your healthcare provider before trying them. \\
\textbf{P:} I understand. I'll make sure to consult with you before trying any alternative treatments. One last question, can asthma be cured? \\
\textbf{D:} Currently, there is no cure for asthma. However, ongoing research is being conducted to better understand the condition and develop new treatments. In the meantime, our goal is to help you manage your symptoms effectively and improve your quality of life. \\
\textbf{P:} Thank you for answering my questions, doctor. I feel more informed now. \\
\textbf{D:} You're welcome. It's important to have all your concerns addressed. Remember, I'm here to support you throughout your asthma management journey. Don't hesitate to reach out if you have any further questions or need assistance. \\
\textbf{P:} I appreciate your support, doctor. I'll be sure to keep in touch. Goodbye. \\
\textbf{D:} Goodbye and take care. \\
%\caption{test}

\end{tcolorbox}
%\vspace{-10mm}
\captionof{figure}{An example of Patient-Doctor conversation.}
\label{box:patient_doctor_conversation}

\begin{tcolorbox}[colback=blue!5!white,colframe=blue!75!black,title=Clinical Summary]
\footnotesize
\textbf{Subjective:} \\
- Symptoms: Shortness of breath, wheezing, cough \\
- Severity: Moderate \\
- Duration: Past week \\
- Associated symptoms: Wheezing, cough \\
- Relevant medical history: Childhood asthma, no recent issues \\
- Family history: Mother had asthma \\
- Allergies: Allergic to pollen \\
- Other concerns: Patient is seeking guidance on asthma management and alternative treatments \\

\textbf{Objective:} \\
- Physical examination findings: Wheezing on auscultation \\
- Spirometry test planned for tomorrow \\
- Blood tests planned for tomorrow \\

\textbf{Assessment:} \\
- Likely diagnosis: Asthma exacerbation \\
- Differential diagnosis: Other conditions that may present with similar symptoms \\
- Clinical impression: Patient has a history of asthma and is experiencing symptoms consistent with an asthma exacerbation \\

\textbf{Plan:} \\
- Spirometry test tomorrow \\
- Blood tests tomorrow \\
- Consider long-acting bronchodilator for daily management \\
- Recommend short-acting bronchodilator for as needed use during episodes of shortness of breath \\
- Discuss proper inhaler technique and asthma management strategies \\
- Consider pre-exercise bronchodilator to prevent exercise-induced symptoms \\
- Emphasize the importance of regular check-ups and monitoring asthma control \\
- Provide education on potential side effects of medications (tremors, increased heart rate, headache) \\
- Recommend annual flu vaccine to reduce risk of respiratory infections \\
- Discuss the importance of avoiding triggers (exposure to allergens or irritants) \\
- Consider alternative treatments with caution \\
\end{tcolorbox}

\captionof{figure}{An example of generated clinical summary.}
\label{box:summary_from_conversation}

\subsection{Illustration}
Imagine if we had the following diarized patient-doctor conversation, 

\begin{tcolorbox}[colback=blue!5!white,colframe=blue!75!black,title=Diarized Patient-Doctor Conversation, breakable]
\footnotesize
\textbf{P:} Good morning, doctor. \\
\textbf{D:} Good morning. What brings you here? \\
\textbf{P:} I've had a cough for about six months. Recently noticed some blood. \\
\textbf{D:} Is it a dry or wet cough? \\
\textbf{P:} Mostly dry. But lately with some blood. \\
\textbf{D:} How much blood are you coughing up? \\
\textbf{P:} About two or three teaspoons a day. \\
\textbf{D:} Any shortness of breath or chest pain? \\
\textbf{P:} Shortness of breath, especially with activity. But no chest pain. \\
\textbf{D:} Any recent weight loss? \\
\textbf{P:} Yes, around ten to fifteen pounds in the last two months. \\
\textbf{D:} Do you smoke? \\
\textbf{P:} Yes, half a pack a day. I've been cutting down. \\
\textbf{D:} We need to do a chest X-ray and sputum test. Lung cancer is a concern given your symptoms and smoking history. \\
\textbf{P:} That makes sense. Thank you. \\
\textbf{D:} We'll proceed with those tests and follow up. Take care. \\
\textbf{P:} Thank you, doctor. Goodbye. \\
\textbf{D:} Goodbye and take care. \\
\end{tcolorbox}

This diarized text can simply be converted to patient-doctor transcribed text like this,

\begin{tcolorbox}[colback=blue!5!white,colframe=blue!75!black,title=Transcribed Patient-Doctor Conversation, breakable]
\footnotesize
Good morning, doctor. Good morning. What brings you here? I've had a cough for about six months. Recently noticed some blood. Is it a dry or wet cough? Mostly dry. But lately with some blood. How much blood are you coughing up? About two or three teaspoons a day. Any shortness of breath or chest pain? Shortness of breath, especially with activity, but no chest pain. Any recent weight loss? Yes, around ten to fifteen pounds in the last two months. Do you smoke? Yes, half a pack a day. I've been cutting down. We need to do a chest X-ray and sputum test. Lung cancer is a concern given your symptoms and smoking history. That makes sense. Thank you. We'll proceed with those tests and follow up. Take care. Thank you, doctor. Goodbye. Goodbye and take care.
\end{tcolorbox}

\subsection*{Retriever Based Filtering}

\textbf{Splitting}

In the first step of retriever-based filtering, we split the transcribed text into individual sentences. This approach ensures that each sentence is processed independently, so the information is contained within each sentence without being spread across multiple chunks. As a result, each chunk makes sense on its own, independent of the others, when received by the LLM.

\begin{tcolorbox}[colback=blue!5!white,colframe=blue!75!black,title=Sentence-wise Splitted Chunked Patient-Doctor Conversation, breakable]
\footnotesize
\textbf{Chunk 1}: Good morning, doctor. \\
\textbf{Chunk 2}: Good morning. \\
\textbf{Chunk 3}: What brings you here? \\
\textbf{Chunk 4}: I've had a cough for about six months. \\
\textbf{Chunk 5}: Recently noticed some blood. \\
\textbf{Chunk 6}: Is it a dry or wet cough? \\
\textbf{Chunk 7}: Mostly dry. \\
\textbf{Chunk 8}: But lately with some blood. \\
\textbf{Chunk 9}: How much blood are you coughing up? \\
\textbf{Chunk 10}: About two or three teaspoons a day. \\
\textbf{Chunk 11}: Any shortness of breath or chest pain? \\
\textbf{Chunk 12}: Shortness of breath, especially with activity. \\
\textbf{Chunk 13}: But no chest pain. \\
\textbf{Chunk 14}: Any recent weight loss? \\
\textbf{Chunk 15}: Yes, around ten to fifteen pounds in the last two months. \\
\textbf{Chunk 16}: Do you smoke? \\
\textbf{Chunk 17}: Yes, half a pack a day. \\
\textbf{Chunk 18}: I've been cutting down. \\
\textbf{Chunk 19}: We need to do a chest X-ray and sputum test. \\
\textbf{Chunk 20}: Lung cancer is a concern given your symptoms and smoking history. \\
\textbf{Chunk 21}: That makes sense. \\
\textbf{Chunk 22}: Thank you. \\
\textbf{Chunk 23}: We'll proceed with those tests and follow up. \\
\textbf{Chunk 24}: Take care. \\
\textbf{Chunk 25}: Thank you, doctor. \\
\textbf{Chunk 26}: Goodbye. \\
\textbf{Chunk 27}: Goodbye and take care.
\end{tcolorbox}

\textbf{Indexing}

After splitting, we embedded each chunk for retrieval handling.

\begin{tcolorbox}[colback=blue!5!white,colframe=blue!75!black,title=Embedded Patient-Doctor Conversation, breakable]
\footnotesize
\textbf{Chunk 1:} \textit{Good morning, doctor.} \\
\textbf{Embedded Format:} \\
\begin{minipage}[t]{0.45\textwidth}
\footnotesize
\begin{verbatim}
[0.123, -0.567, 0.910...]
\end{verbatim}
\end{minipage}

\textbf{Chunk 2:} \textit{Good morning.} \\
\textbf{Embedded Format:} \\
\begin{minipage}[t]{0.45\textwidth}
\footnotesize
\begin{verbatim}
[0.234, -0.678, 0.821...]
\end{verbatim}
\end{minipage}

\textbf{Chunk 3:} \textit{What brings you here?} \\
\textbf{Embedded Format:} \\
\begin{minipage}[t]{0.45\textwidth}
\footnotesize
\begin{verbatim}
[0.345, -0.789, 0.732...]
\end{verbatim}
\end{minipage}

\textbf{Chunk 4:} \textit{I've had a cough for about six months.} \\
\textbf{Embedded Format:} \\
\begin{minipage}[t]{0.45\textwidth}
\footnotesize
\begin{verbatim}
[0.456, -0.890, 0.643...]
\end{verbatim}
\end{minipage}

\textbf{Chunk 5:} \textit{Recently noticed some blood.} \\
\textbf{Embedded Format:} \\
\begin{minipage}[t]{0.45\textwidth}
\footnotesize
\begin{verbatim}
[0.567, -0.901, 0.554...]
\end{verbatim}
\end{minipage}

\textbf{Chunk 6:} \textit{Is it a dry or wet cough?} \\
\textbf{Embedded Format:} \\
\begin{minipage}[t]{0.45\textwidth}
\footnotesize
\begin{verbatim}
[0.678, -0.912, 0.465...]
\end{verbatim}
\end{minipage}

\textbf{Chunk 7:} \textit{Mostly dry.} \\
\textbf{Embedded Format:} \\
\begin{minipage}[t]{0.45\textwidth}
\footnotesize
\begin{verbatim}
[0.789, -0.923, 0.376...]
\end{verbatim}
\end{minipage}

\textbf{Chunk 8:} \textit{But lately with some blood.} \\
\textbf{Embedded Format:} \\
\begin{minipage}[t]{0.45\textwidth}
\footnotesize
\begin{verbatim}
[0.890, -0.934, 0.287...]
\end{verbatim}
\end{minipage}

\textbf{Chunk 9:} \textit{How much blood are you coughing up?} \\
\textbf{Embedded Format:} \\
\begin{minipage}[t]{0.45\textwidth}
\footnotesize
\begin{verbatim}
[0.901, -0.945, 0.198...]
\end{verbatim}
\end{minipage}

\textbf{Chunk 10:} \textit{About two or three teaspoons a day.} \\
\textbf{Embedded Format:} \\
\begin{minipage}[t]{0.45\textwidth}
\footnotesize
\begin{verbatim}
[0.012, -0.956, 0.109...]
\end{verbatim}
\end{minipage}

\textbf{Chunk 11:} \textit{Any shortness of breath or chest pain?} \\
\textbf{Embedded Format:} \\
\begin{minipage}[t]{0.45\textwidth}
\footnotesize
\begin{verbatim}
[0.123, -0.967, 0.210...]
\end{verbatim}
\end{minipage}

\textbf{Chunk 12:} \textit{Shortness of breath, especially with activity.} \\
\textbf{Embedded Format:} \\
\begin{minipage}[t]{0.45\textwidth}
\footnotesize
\begin{verbatim}
[0.234, -0.978, 0.321...]
\end{verbatim}
\end{minipage}

\textbf{Chunk 13:} \textit{But no chest pain.} \\
\textbf{Embedded Format:} \\
\begin{minipage}[t]{0.45\textwidth}
\footnotesize
\begin{verbatim}
[0.345, -0.989, 0.432...]
\end{verbatim}
\end{minipage}

\textbf{Chunk 14:} \textit{Any recent weight loss?} \\
\textbf{Embedded Format:} \\
\begin{minipage}[t]{0.45\textwidth}
\footnotesize
\begin{verbatim}
[0.456, -0.990, 0.543...]
\end{verbatim}
\end{minipage}

\textbf{Chunk 15:} \textit{Yes, around ten to fifteen pounds in the last two months.} \\
\textbf{Embedded Format:} \\
\begin{minipage}[t]{0.45\textwidth}
\footnotesize
\begin{verbatim}
[0.567, -0.991, 0.654...]
\end{verbatim}
\end{minipage}

\textbf{Chunk 16:} \textit{Do you smoke?} \\
\textbf{Embedded Format:} \\
\begin{minipage}[t]{0.45\textwidth}
\footnotesize
\begin{verbatim}
[0.678, -0.992, 0.765...]
\end{verbatim}
\end{minipage}

\textbf{Chunk 17:} \textit{Yes, half a pack a day.} \\
\textbf{Embedded Format:} \\
\begin{minipage}[t]{0.45\textwidth}
\footnotesize
\begin{verbatim}
[0.789, -0.993, 0.876...]
\end{verbatim}
\end{minipage}

\textbf{Chunk 18:} \textit{I've been cutting down.} \\
\textbf{Embedded Format:} \\
\begin{minipage}[t]{0.45\textwidth}
\footnotesize
\begin{verbatim}
[0.890, -0.994, 0.987...]
\end{verbatim}
\end{minipage}

\textbf{Chunk 19:} \textit{We need to do a chest X-ray and sputum test.} \\
\textbf{Embedded Format:} \\
\begin{minipage}[t]{0.45\textwidth}
\footnotesize
\begin{verbatim}
[0.901, -0.995, 0.098...]
\end{verbatim}
\end{minipage}

\textbf{Chunk 20:} \textit{Lung cancer is a concern given your symptoms and smoking history.} \\
\textbf{Embedded Format:} \\
\begin{minipage}[t]{0.45\textwidth}
\footnotesize
\begin{verbatim}
[0.012, -0.996, 0.209...]
\end{verbatim}
\end{minipage}

\textbf{Chunk 21:} \textit{That makes sense.} \\
\textbf{Embedded Format:} \\
\begin{minipage}[t]{0.45\textwidth}
\footnotesize
\begin{verbatim}
[0.123, -0.997, 0.320...]
\end{verbatim}
\end{minipage}

\textbf{Chunk 22:} \textit{Thank you.} \\
\textbf{Embedded Format:} \\
\begin{minipage}[t]{0.45\textwidth}
\footnotesize
\begin{verbatim}
[0.125, -0.897, 0.356...]
\end{verbatim}
\end{minipage}

\textbf{Chunk 23:} \textit{We'll proceed with those tests and follow up.} \\
\textbf{Embedded Format:} \\
\begin{minipage}[t]{0.45\textwidth}
\footnotesize
\begin{verbatim}
[0.234, -0.998, 0.431...]
\end{verbatim}
\end{minipage}

\textbf{Chunk 24:} \textit{Take care.} \\
\textbf{Embedded Format:} \\
\begin{minipage}[t]{0.45\textwidth}
\footnotesize
\begin{verbatim}
[0.345, -0.999, 0.542...]
\end{verbatim}
\end{minipage}

\textbf{Chunk 25:} \textit{Thank you, doctor.} \\
\textbf{Embedded Format:} \\
\begin{minipage}[t]{0.45\textwidth}
\footnotesize
\begin{verbatim}
[-0.345, -0.934, 0.542...]
\end{verbatim}
\end{minipage}

\textbf{Chunk 26:} \textit{Goodbye.} \\
\textbf{Embedded Format:} \\
\begin{minipage}[t]{0.45\textwidth}
\footnotesize
\begin{verbatim}
[0.356, -0.999, 0.532...]
\end{verbatim}
\end{minipage}

\textbf{Chunk 27:} \textit{Goodbye and take care.} \\
\textbf{Embedded Format:} \\
\begin{minipage}[t]{0.45\textwidth}
\footnotesize
\begin{verbatim}
[0.344, -0.999, -0.742...]
\end{verbatim}
\end{minipage}

\vspace{5mm}
\textit{Note: The embedding values shown are illustrative representations and not actual embedding values.}
\end{tcolorbox}

\textbf{Retrieval}

Now, we embed the retriever query and use it to identify the relevant embedded chunks for generating SOAP notes.

\begin{tcolorbox}[colback=blue!5!white,colframe=blue!75!black,title=Retrived and Rearranged Chunks, breakable]
\footnotesize

\textbf{Retrieved Chunk 1: } \\
\begin{minipage}[t]{0.45\textwidth}
\footnotesize
\begin{verbatim}
[0.456, -0.890, 0.643...]
\end{verbatim}
\end{minipage}

\textbf{Retrieved Chunk 2: } \\
\begin{minipage}[t]{0.45\textwidth}
\footnotesize
\begin{verbatim}
[0.567, -0.901, 0.554...]
\end{verbatim}
\end{minipage}

\textbf{Retrieved Chunk 3: } \\
\begin{minipage}[t]{0.45\textwidth}
\footnotesize
\begin{verbatim}
[0.678, -0.912, 0.465...]
\end{verbatim}
\end{minipage}

\textbf{Retrieved Chunk 4: } \\
\begin{minipage}[t]{0.45\textwidth}
\footnotesize
\begin{verbatim}
[0.789, -0.923, 0.376...]
\end{verbatim}
\end{minipage}

\textbf{Retrieved Chunk 5: } \\
\begin{minipage}[t]{0.45\textwidth}
\footnotesize
\begin{verbatim}
[0.890, -0.934, 0.287...]
\end{verbatim}
\end{minipage}

\textbf{Retrieved Chunk 6: } \\
\begin{minipage}[t]{0.45\textwidth}
\footnotesize
\begin{verbatim}
[0.901, -0.945, 0.198...]
\end{verbatim}
\end{minipage}

\textbf{Retrieved Chunk 7: } \\
\begin{minipage}[t]{0.45\textwidth}
\footnotesize
\begin{verbatim}
[0.012, -0.956, 0.109...]
\end{verbatim}
\end{minipage}

\textbf{Retrieved Chunk 8: } \\
\begin{minipage}[t]{0.45\textwidth}
\footnotesize
\begin{verbatim}
[0.123, -0.967, 0.210...]
\end{verbatim}
\end{minipage}

\textbf{Retrieved Chunk 9: } \\
\begin{minipage}[t]{0.45\textwidth}
\footnotesize
\begin{verbatim}
[0.234, -0.978, 0.321...]
\end{verbatim}
\end{minipage}

\textbf{Retrieved Chunk 10: } \\
\begin{minipage}[t]{0.45\textwidth}
\footnotesize
\begin{verbatim}
[0.345, -0.989, 0.432...]
\end{verbatim}
\end{minipage}

\textbf{Retrieved Chunk 11: } \\
\begin{minipage}[t]{0.45\textwidth}
\footnotesize
\begin{verbatim}
[0.456, -0.990, 0.543...]
\end{verbatim}
\end{minipage}

\textbf{Retrieved Chunk 12: } \\
\begin{minipage}[t]{0.45\textwidth}
\footnotesize
\begin{verbatim}
[0.567, -0.991, 0.654...]
\end{verbatim}
\end{minipage}

\textbf{Retrieved Chunk 13: } \\
\begin{minipage}[t]{0.45\textwidth}
\footnotesize
\begin{verbatim}
[0.678, -0.992, 0.765...]
\end{verbatim}
\end{minipage}

\textbf{Retrieved Chunk 14: } \\
\begin{minipage}[t]{0.45\textwidth}
\footnotesize
\begin{verbatim}
[0.789, -0.993, 0.876...]
\end{verbatim}
\end{minipage}

\textbf{Retrieved Chunk 15: } \\
\begin{minipage}[t]{0.45\textwidth}
\footnotesize
\begin{verbatim}
[0.890, -0.994, 0.987...]
\end{verbatim}
\end{minipage}

\textbf{Retrieved Chunk 16: } \\
\begin{minipage}[t]{0.45\textwidth}
\footnotesize
\begin{verbatim}
[0.901, -0.995, 0.098...]
\end{verbatim}
\end{minipage}

\textbf{Retrieved Chunk 17: } \\
\begin{minipage}[t]{0.45\textwidth}
\footnotesize
\begin{verbatim}
[0.012, -0.996, 0.209...]
\end{verbatim}
\end{minipage}

\vspace{5mm}
\textit{Note: The above chunks are retrieved with respect to query embedding; [0.321, -0.654, 0.789...] by hybrid retriever and then done RRF on it.}
\end{tcolorbox}

We then decode each chunk into its string format and concatenate them to serve as context for generating SOAP notes.

\begin{tcolorbox}[colback=blue!5!white,colframe=blue!75!black,title=Retrived information from the Patient-Doctor Conversation which is Relevent for Generating SOAP Notes, breakable]
\footnotesize
I've had a cough for about six months. Recently, I've noticed some blood. Is it a dry or wet cough? It's mostly dry. But lately, there's been some blood. How much blood are you coughing up? About two or three teaspoons a day. Any shortness of breath or chest pain? Yes, there's shortness of breath, especially with activity. But no chest pain. Any recent weight loss? Yes, around ten to fifteen pounds in the last two months. Do you smoke? Yes, half a pack a day. I've been cutting down. We need to do a chest X-ray and sputum test. Lung cancer is a concern given your symptoms and smoking history.
\end{tcolorbox}

\subsection*{Inference}

We then pass the output from the retriever-based filtering, along with the LLM query, to the LLM (whether fine-tuned or not) to generate the SOAP notes.

\begin{tcolorbox}[colback=blue!5!white,colframe=blue!75!black,title=SOAP Note]
\footnotesize
\textbf{Subjective:} \\
- Chief Complaint: Persistent cough for six months, with recent onset of blood in sputum \\
- Cough: Mostly dry, with blood present (approximately two to three teaspoons daily) \\
- Shortness of Breath: Noted, particularly with activity \\
- Chest Pain: None reported \\
- Weight Loss: Significant loss of 10-15 pounds over the past two months \\
- Smoking History: Current smoker, approximately half a pack per day; attempting to reduce \\

\textbf{Objective:} \\
- General Appearance: Weight loss evident \\
- Respiratory: Dry cough with recent hemoptysis. Shortness of breath noted on exertion \\
- Vital Signs: [To be completed based on actual values] \\
- Physical Exam: [To be completed based on findings, if available] \\

\textbf{Assessment:} \\
- Primary Concern: Hemoptysis with chronic cough, significant weight loss, shortness of breath, and smoking history raise concern for possible lung cancer \\
- Differential Diagnosis: Lung cancer, chronic bronchitis, tuberculosis, or other respiratory pathology \\

\textbf{Plan:} \\
- Immediate Actions: \\
  - Order Chest X-ray to assess for possible malignancy or other abnormalities \\
  - Request Sputum Test to evaluate for infectious or malignant cells \\
- Follow-Up: Schedule a follow-up appointment to review test results and determine further management \\
- Patient Education: Discuss the importance of smoking cessation and provide resources for support in quitting \\
\end{tcolorbox}

\captionof{figure}{An example of a SOAP note summarizing patient symptoms and management plan.}
\label{box:soap_note}

%and need to select which SOAP summary you prefer the most between 3 (highlighted in different colors in Column A, Column B, and Column C).
